# Supplementary material for: Constraint Inference in Control Tasks from Expert Demonstrations via Inverse Optimization
Source: arXiv:2304.03367 source file (2023-12-04)
Supplement: Supplementary file 1 [file appendix.tex]

\appendix

\section{Cumulative Greedy Constraint Inference}
Algorithm~\ref{alg:al_greedy} considers each time the addition of one individual linear constraints and depending on the evaluation of the KKT residual objective function that constraints is added in the list of inferred constraints. This has the potential downside of a wrongly inferred constraints affecting inference for future constraints. 

\begin{algorithm}[H]
\caption{Cumulative Greedy Constraint Inference (CGCI)}\label{alg:al_greedy2}
\textbf{Input:} Stopping criterion $Obj_{thr}$\\
\textbf{Initialize:} $C_{set}=\{\}$, $Obj_{list} =\{\text{Large Number}\}$\\
\For{$N =1,\ldots$}{
Obtain $c\in\mathbb{R}^{NT}$ from Algorithm~\ref{alg:alg_alter}\\
\eIf{$|Objective-Obj_{list}(N)|\geq Obj_{thr}$ }
    {
       break
    }
    {$Obj_{list}(N)\gets Objective$
    }
}
\textbf{Output:} $c$
\end{algorithm}

Algorithm~\ref{alg:al_greedy2} considers each time a different number of potential constraints and infers all of them via Algorithm~\ref{algo:alter} at once. As the correct number of constraints is expected to produce the smaller objective function, the process terminates once the objective function starts increasing.

\section{Nonlinear Constraints}\label{sec:nonl_cnstr}

Although the main target of this work lies in inferring linear constraints from expert demonstrations, the case of nonlinear constrains can also be tackled via Algorithm~\ref{algo:alter}.  In this section, we investigate constraint inference of nonlinear constraints, both convex and non-convex. The forward optimal control task with generic convex constraints can be written as follows
\begin{equation}\label{prob:lqr_cvx_cnstr}
    \begin{aligned}
    \min_{\{x_t,u_t\}_{t=0}^{t=T}}& \sum_{t=0}^{T} x_t^\top Q x_t + u_t^\top R u_t \\
    \textrm{s.t. }& x_{t+1} = A x_t + B u_t, \forall t\in\{1,\dots, T-1\},\\
    & g(x_t) \leq 0, \forall t \in \{1,\dots,T\},
    \end{aligned}
\end{equation}
with $g(x_t)$ being a nonlinear function. In this framework, the KKT conditions become

\begin{equation}
    \begin{aligned}
        &\nabla_U L(U,\lambda) = 2G^\top (I_T\otimes Q)(GU+Hx_0-X_{track})+2 (I_T\otimes R)U\\
        &+2\sum_{i=1}^T\lambda_i\nabla_Ug(x_i)=0 \\ 
        &\sum_{i=1}^T\lambda_i g(x_i)=0\\
        &g(x_i)\le 0, \;i=1,\ldots,T\\
        &\lambda\ge 0.
    \end{aligned}
\end{equation}

Nonlinear constraints trivially lead to nonlinear inverse problems. In what follows we will examine two cases, one in which $g(\cdot)$ is a convex parabolic function and one in which it is non-convex norm constraint, and propose methods to obtain estimates of the unknown constraints in both cases.

\subsection{Convex Parabolic Constraints}
In this section we consider convex nonlinear constraints of parabolic form, as these constitute a broad family of nonlinear constraints.  The constraint function now has the form

\begin{align}\label{eq:parabolic_cnstr}
g(x_i)= x_i^{\top}Px_i+Sx_i+c
\end{align}
where $P\in\mathbb{R}^{n\times n}$ and $S\in\mathbb{R}^n$. The Lagrangian takes the form
\begin{equation}
\begin{aligned}
    L(U,\lambda):=&(GU+Hx_0-X_{track})^\top (I_T\otimes Q)(GU+Hx_0-X_{track})+U^\top (I_T\otimes R)U\\
    &+\sum_i\lambda_i (x_i^{\top}Px_i+Sx_i+c)
\end{aligned}
\end{equation}
and the KKT conditions now become
\begin{equation}
\begin{aligned}
    &\nabla_U L(U,\lambda) = 2G^\top (I_T\otimes Q)(GU+Hx_0-X_{track})+2 (I_T\otimes R)U\\
    &+2\sum_i\lambda_i2Px_i=0 \\ 
    &\sum_i\lambda_i (x_i^{\top}Px_i+Sx_i+c)=0\\
    &g(x_i)\le 0, i=1,\ldots,T\\
    &\lambda\ge 0.
\end{aligned}
\end{equation}

\subsection{Non-Convex Parabolic Constraints}
We also specifically investigate the case of non-convex parabolic constraints which are commonly used for obstacle avoidance  in robot navigation tasks~\cite{sundar1997optimal}.
% Consider the compact version problem:
% \begin{equation}
%     \begin{aligned}
%     \min_{U\in \mathbb{R}^{Tm}}& (GU+Hx_0-X_{track})^\top (I_T\otimes Q)(GU+Hx_0-X_{track})+U^\top (I_T\otimes R)U\\
%     \textrm{s.t. }& ||G_iU+H_ix_0-x_c||_2^2\le r^2,\;\;\; i=1,
%     \ldots, T
%     \end{aligned}
% \end{equation}
% where $G_i$ denotes the $i$th row of the matrix and $x_c$ and $r$ denote the center and radius of a circle, respectively. We have the Lagrangian
% \begin{equation}
% \begin{aligned}
%     L(U,\lambda):=&(GU+Hx_0-X_{track})^\top (I_T\otimes Q)(GU+Hx_0-X_{track})+U^\top (I_T\otimes R)U\\
%     &+\sum_i\lambda_i (|| G_iU+H_ix_0-x_c)||_2^2-r^2)
% \end{aligned}
% \end{equation}
% The KKT conditions are
% \begin{equation}
% \left\{\begin{aligned}
%     &\nabla_U L(U,\lambda) = 2G^\top (I_T\otimes Q)(GU+Hx_0-X_{track})+2 (I_T\otimes R)U+2\sum_i\lambda_iG_i^{\top}(G_iU+H_ix_0-x_c)=0 \\ 
%     &\sum_i\lambda_i (|| G_iU+H_ix_0-x_c)||_2^2-r^2)=0\\
%     &|| G_iU+H_ix_0-x_c)||_2^2-r^2\le 0, i=1,\ldots,T\\
%     &\lambda\ge 0
% \end{aligned}\right.
% \end{equation}
In this case, $g(\cdot)$ has the same for as in~\eqref{eq:parabolic_cnstr} with the only difference being that $P$ is no longer positive semi-definite. This for of constraints includes norm constraints of the form $||G_iU+H_ix_0-x_c||_2^2\geq r^2, i=1,\ldots,T$, where $G_i$ denotes the $i$th row of the matrix and $x_c$ designates the center of the ball from which a minimum distance of $r$ must be maintained during the control task.
% \begin{equation}
% \begin{aligned}
%     L(U,\lambda):=&(GU+Hx_0-X_{track})^\top (I_T\otimes Q)(GU+Hx_0-X_{track})+U^\top (I_T\otimes R)U\\
%     &+\sum_i\lambda_i (|| G_iU+H_ix_0-x_c)||_2^2-r^2).
% \end{aligned}
% \end{equation}
% The KKT conditions are
% \begin{equation}
% \left\{\begin{aligned}
%     &\nabla_U L(U,\lambda) = 2G^\top (I_T\otimes Q)(GU+Hx_0-X_{track})+2 (I_T\otimes R)U\\
%     &+2\sum_i\lambda_iG_i^{\top}(G_iU+H_ix_0-x_c)=0 \\ 
%     &\sum_i\lambda_i (|| G_iU+H_ix_0-x_c)||_2^2-r^2)=0\\
%     &|| G_iU+H_ix_0-x_c)||_2^2-r^2\le 0, i=1,\ldots,T\\
%     &\lambda\ge 0.
% \end{aligned}\right.
% \end{equation}
It should be noted that in this case Algorithm~\ref{algo:alter} can still be utilized. However, the individual subproblem that solves for $x_c$ and $r$ is no longer a convex problem and a nonlinear solver must be utilized for this step of the alternating optimization.

\section{Nonlinear Constraints Simulations}
This section constraints simulations regarding constraint inference for convex and non-convex constraints. 

\subsection{Convex Parabolic Constraints}
We consider two dimensional convex parabolic constraints of the form $g(x_i)=x_{i,1}-1+(x_{i,2}+1)^2$, with the $i,j$ denoting the $j$th coordinate of state $i$.

\subsection{Non-Convex Constraints}

 In the non-convex constraint case we consider norm constraints of the form $g(x_i)=-||x_i-x_c||_2^2 + r^2, i=1,\ldots,T$, that require from the agent to keep a certain distance from an obstacle.

% \subsection{General Nonlinear Constraints}

% This section studies the more general case in which the constraints can be a generic nonlinear function, and hence the constraint can be non-convex. The trajectory planning optimization problem solved is

% \begin{equation}\label{eq:gen_opt}
%     \begin{aligned}
%     &\min_{u_t} \sum_t f(x_t,u_t)\\
%     & \textrm{s.t. } g(x_t,u_t) \leq {{0} }, \forall t
%     \end{aligned}
% \end{equation}

\section{Simulation Details}
All the simulations were carried out in a two dimensional space $x_t\in\mathbb{R}^2$.

\subsection{Two Constraints}
In the two constraint case we used a horizon $T=8$, a starting state $x_0=(0.5,-5.5)$ and we requested from the controller to follow the trajectory $x_{traj}=[(0,-5.5),(-0.6,-4.5),(-1,-3.8),$ $(-1.5,-3.5),(-1.6,-2.5),(-0.2,-2),(0.5,-2),(0.8,-2)]$. To collect multiple trajectories we added each time Gaussian noise $\mathcal{N}(0,1)$ to each initial state dimension.  The original constraints are $c_1:$ and $c_2:$.

\subsection{Three Constraints}

In the three constraint case we used a horizon $T=12$, a starting state $x_0=(-2,-15)$ and we requested from the controller to follow the trajectory $x_{traj}=[(-3.5,-4),(-3.0,-3),(-2.5,-2),$ $(-2,-1),(-1.5,-1),(0.5,0),(1.5,1),(2,1),(2,1),(2,1),(2,1)]$. To collect multiple trajectories we added each time Gaussian noise $\mathcal{N}(0,1)$ to each initial state dimension.  The original constraints are $c_1:$, $c_2:$ and $c_3:$

% \begin{table}[H]
% \centering
% \begin{tabular}{ ccccccc } 
% & \multicolumn{2}{c}{N} & \multicolumn{2}{c}{T}\\ \cmidrule(lr){2-3} \cmidrule(lr){4-5}
%  %\thickhline
%  2 constraints &  4 & - & - & -   \\ 
% 3 constraints &  - & - & - & - & - & - \\ 
%  \thickhline
% %$4$ & $0.36$ & $0.37$ & -$0.65$ & -$0.18$ & -$0.09$ &\bftab{0.36}\\ 
% %  $1000$ & ${0.34}$ & $0.38$ & ${0.12}$ & $\textbf{0.26}$ & $\textbf{0.35}$ & $\textbf{0.15}$   \\ 
% %  $5000$ & ${0.25}$ & $\textbf{0.13}$ & ${0.23}$ & $\textbf{0.08}$ & $0.2$ & $\textbf{0.46}$  \\ 
% %  $10000$ & $0.12$ & $\textbf{0.08}$ & $0.43$ & $\textbf{0.03}$ & ${0.11}$ & $\textbf{0.67}$ \\ 
%  \thickhline
% \end{tabular}
% \label{table:averaged_metrics_comparison}
% \caption{TB}
% \end{table}

% \section{Remarks}
% \textbf{10/14}
% \begin{enumerate}
% \item convergence in optimal solution biconvex problems
% \item Show simple case is hard and has high complexity, multiple local minima
% \end{enumerate}
